# Supplementary material for: Giant resonant nonlinear damping in nanoscale ferromagnets
Source: arXiv:1803.10925 source file (2018-03-29)
Supplement: Supplementary file 1 [file supplemental.pdf]

# Supplemental Material:
# Giant resonant nonlinear damping in nanoscale ferromagnets

I. Barsukov,[1] H. K. Lee,[1] A. A. Jara,[1] Y.-J. Chen,[1] A. M. Gonçalves,[1] C. Sha,[1] J. A. Katine,[2] R. E. Arias,[3] B. A. Ivanov,[4,5] and I. N. Krivorotov[1]

[1] *Physics and Astronomy, University of California, Irvine, CA 92697, USA*
[2] *Western Digital, 5600 Great Oaks Parkway, San Jose, CA 95119, USA*
[3] *Departamento de Física, CEDENNA, FCFM, Universidad de Chile, Santiago, Chile*
[4] *Institute of Magnetism, National Academy of Sciences of Ukraine, Vernadsky av. 36 B, Kyiv, 03142, Ukraine*
[5] *National University of Science and Technology MISiS, Moscow, 119049, Russian Federation*

## I. METHODS

### A. Linewidth evaluation

All measurements presented were carried out with magnetic field applied along the easy axis of the MTJ devices so that the magnetic moments of the free and pinned layers are collinear to each other. In this geometry, the ST-FMR signals are dominated by photo-resistance contribution and are proportional to the square of the transverse component of the dynamic magnetization magnetization [1], which allows us to directly compare calculated $|a|^2(\omega)$ resonance curves to measured ST-FMR resonance curves $\tilde{V}_{\rm mix}(f)$ and to $V_{\rm mix}(f)$ approximated by numerical integration $\int \tilde{V}_{\rm mix}(f){\rm d}f$.

When $V_{\rm mix}(f)$ and $|a|^2(\omega)$ are single-peak curves, they are fit to a sum of symmetric and antisymmetric Lorentzian curves with identical central frequencies and linewidth parameters as described in Ref. [2], and the spectral linewidth is determined as half-width at the half-maximum of the symmetric Lorentzian curve.

In order to quantify the linewidth of the split-peak resonance profile, we introduce a fitting function that is a sum of two Lorentzian curves with different central frequencies separated by $\delta f$. The half width of the resonance profile $\Delta f_0$ is then defined as the average of the half widths of the two Lorentzians plus $\delta f/2$.

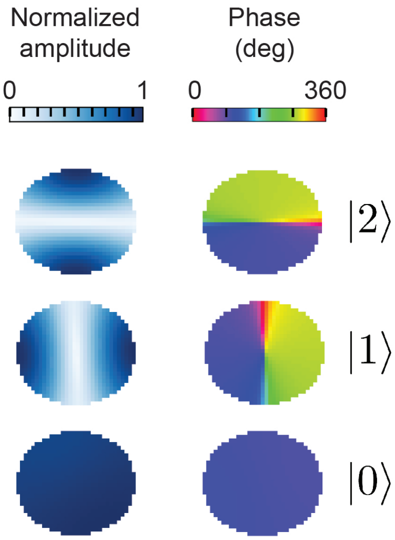


Supplemental Figure 1. Spatial profiles of spin wave eigenmodes. Normalized amplitude and phase of the three lowest frequency spin wave eigenmodes of the MTJ free layer, given by micromagnetic simulations.

### B. Micromagnetic simulations

Micromagnetic simulations were performed using OOMMF software [3, 4]. To account for all magnetic interactions in the MTJ, a three dimensional model was employed with three ferromagnetic layers: free, SAF top and SAF bottom. We use material parameters obtained from the measurements and/or their accepted literature values (see Ref. [2] for

the MTJ structure and fabrication details). Magnetization dynamics is excited by a combined pulse of spin torque and Oersted field, resulting from a sinc-shaped spatially uniform current pulse. The spatial profile of the Oersted field corresponds to that of a long wire with elliptical cross section. The direction of the spin torque vector acting on the free layer is determined by the magnetization orientation of the SAF top layer. The spectrum of spin wave eigenmodes is obtained via fast Fourier transform (FFT) of the time dependent components of the layers' magnetic moment. Spatial mapping of the resulting Fourier amplitude and phase at a given frequency provides the mode profiles (Supplmental Fig. 1). The observed excitations are confirmed to be spin wave modes localized to the free layer. SAF modes are found at much higher frequencies than the free layer modes, and their frequencies are found to be incommensurable to the free layer quasi-uniform mode frequency [5].

## II. SOLUTION OF THE EQUATIONS OF MOTION

The Hamiltonian equations of motion describing the coupled dissipative dynamics of the quasi-uniform ($a$) and the higher-order ($b$) spin wave modes are:

$$i\frac{\mathrm{d}a}{\mathrm{d}t} = \frac{\partial \mathcal{H}}{\partial a^\dagger} + \frac{\partial \mathcal{Q}}{\partial(\mathrm{d}a^\dagger/\mathrm{d}t)} \tag{1}$$

$$i\frac{\mathrm{d}b}{\mathrm{d}t} = \frac{\partial \mathcal{H}}{\partial b^\dagger} + \frac{\partial \mathcal{Q}}{\partial(\mathrm{d}b^\dagger/\mathrm{d}t)} \tag{2}$$

where $\mathcal{H}$ is the Hamiltonian of the system and $\mathcal{Q}$ is the dissipation function, given by:

$$\mathcal{H} = \omega_0 a^\dagger a + \omega_n b^\dagger b + \frac{1}{2}\Psi_0 a^\dagger a^\dagger a a + \frac{1}{2}\Psi_n b^\dagger b^\dagger b b + (\psi_n^* a a b^\dagger + \psi_n a^\dagger a^\dagger b) + \zeta\{\exp(-i\omega t)a^\dagger + \exp(i\omega t)a\} \tag{3}$$

$$\mathcal{Q} = \frac{\mathrm{d}a^\dagger}{\mathrm{d}t}\frac{\mathrm{d}a}{\mathrm{d}t}(\alpha_0 + \eta_0 a^\dagger a) + \frac{\mathrm{d}b^\dagger}{\mathrm{d}t}\frac{\mathrm{d}b}{\mathrm{d}t}(\alpha_n + \eta_n b^\dagger b) \tag{4}$$

By using Eq. (3) and Eq. (4) in Eq. (1) and Eq. (2), the Hamiltonian equations can be written as:

$$i\frac{\mathrm{d}a}{\mathrm{d}t} - (\alpha_0 + \eta_0 a^\dagger a)\frac{\mathrm{d}a}{\mathrm{d}t} = \omega_0 a + 2\psi_n a^\dagger b + \Psi_0 a^\dagger a a + \zeta\exp(-i\omega t) \tag{5}$$

$$i\frac{\mathrm{d}b}{\mathrm{d}t} - (\alpha_n + \eta_n b^\dagger b)\frac{\mathrm{d}b}{\mathrm{d}t} = \omega_n b + \psi_n^* a a + \Psi_n b^\dagger b b \tag{6}$$

Using a periodic ansatz $a = \bar{a}\exp(-i\omega t)$ and $b = \bar{b}\exp(-2i\omega t)$ in Eq. (5) and Eq. (6), where $\bar{a}$ and $\bar{b}$ are complex amplitudes, reduces the Hamiltonian equations to a set of two algebraic equation for the complex amplitudes:

$$\big(\omega - \omega_0 - \Psi_0|\bar{a}|^2 + i(\alpha_0 + \eta_0|\bar{a}|^2)\omega\big)\,\bar{a} - 2\psi_n\bar{a}^*\bar{b} = \zeta \tag{7}$$

$$\big(2\omega - \omega_n - \Psi_n|\bar{b}|^2 + 2i(\alpha_n + \eta_n|\bar{b}|^2)\omega\big)\,\bar{b} = \psi_n^*\bar{a}^2 \tag{8}$$

We solve Eq. (8) for $\bar{b}$ and multiply the numerator and denominator of this expression by the complex conjugate of the denominator:

$$\bar{b} = \psi_n^*\bar{a}^2\frac{\big(2\omega - \omega_n - \Psi_n|\bar{b}|^2\big) - i2(\alpha_n + \eta_n|\bar{b}|^2)\omega}{\big(2\omega - \omega_n - \Psi_n|\bar{b}|^2\big)^2 + 4(\alpha_n + \eta_n|\bar{b}|^2)^2\omega^2} \tag{9}$$

then we multiply Eq. (9) by $\frac{2\psi_n\bar{a}^*}{\bar{a}}$ and evaluate the real and imaginary parts.

$$\Re\left[\frac{2\psi_n\bar{a}^*\bar{b}}{\bar{a}}\right] = |\psi_n|^2|\bar{a}|^2\frac{2\left(2\omega - \omega_n - \Psi_n|\bar{b}|^2\right)}{\big(2\omega - \omega_n - \Psi_n|\bar{b}|^2\big)^2 + 4(\alpha_n + \eta_n|\bar{b}|^2)^2\omega^2} \tag{10}$$

$$\Im\left[\frac{2\psi_n\bar{a}^*\bar{b}}{\bar{a}}\right] = |\psi_n|^2|\bar{a}|^2\frac{-4(\alpha_n + \eta_n|\bar{b}|^2)\omega}{\big(2\omega - \omega_n - \Psi_n|\bar{b}|^2\big)^2 + 4(\alpha_n + \eta_n|\bar{b}|^2)^2\omega^2} \tag{11}$$

By taking the modulus of Eq. (8), we obtain:

$$|\bar{a}|^2 = \frac{|\bar{b}|}{|\psi_n|}\sqrt{\big(2\omega - \omega_n - \Psi_n|\bar{b}|^2\big)^2 + 4(\alpha_n + \eta_n|\bar{b}|^2)^2\omega^2} \tag{12}$$

Using Eq. (12) in Eqs. (10-11), we derive:

$$\Re\left[\frac{2\psi_n \bar{a}^* \bar{b}}{\bar{a}}\right] = \frac{2\left(2\omega-\omega_n-\Psi_n|\bar{b}|^2\right)|\psi_n||\bar{b}|}{\sqrt{\left(2\omega-\omega_n-\Psi_n|\bar{b}|^2\right)^2+4(\alpha_n+\eta_n|\bar{b}|^2)^2\omega^2}} \tag{13}$$

$$\Im\left[\frac{2\psi_n \bar{a}^* \bar{b}}{\bar{a}}\right] = \frac{-4(\alpha_n+\eta_n|\bar{b}|^2)\omega|\psi_n||\bar{b}|}{\sqrt{\left(2\omega-\omega_n-\Psi_n|\bar{b}|^2\right)^2+4(\alpha_n+\eta_n|\bar{b}|^2)^2\omega^2}} \tag{14}$$

Taking the modulus squared of Eq. (7):

$$\left\{\left(\omega-\omega_0-\Psi_0|\bar{a}|^2-\Re\left[\frac{2\psi_n \bar{a}^* \bar{b}}{\bar{a}}\right]\right)^2+\left((\alpha_0+\eta_0|\bar{a}|^2)\omega-\Im\left[\frac{2\psi_n \bar{a}^* \bar{b}}{\bar{a}}\right]\right)^2\right\}|\bar{a}|^2=\zeta^2 \tag{15}$$

and using Equations (12)–(14) in Eq. (15) gives us an algebraic equation for the absolute value of the higher order mode amplitude $|\bar{b}|$:

$$\left\{\left(\omega-\omega_0-\Psi_0\frac{|\bar{b}|}{|\psi_n|}\sqrt{\left(2\omega-\omega_n-\Psi_n|\bar{b}|^2\right)^2+4(\alpha_n+\eta_n|\bar{b}|^2)^2\omega^2}-\frac{2\left(2\omega-\omega_n-\Psi_n|\bar{b}|^2\right)|\psi_n||\bar{b}|}{\sqrt{\left(2\omega-\omega_n-\Psi_n|\bar{b}|^2\right)^2+4(\alpha_n+\eta_n|\bar{b}|^2)^2\omega^2}}\right)^2+\right.$$
$$\left.\left(\left(\alpha_0+\eta_0\frac{|\bar{b}|}{|\psi_n|}\sqrt{\left(2\omega-\omega_n-\Psi_n|\bar{b}|^2\right)^2+4(\alpha_n+\eta_n|\bar{b}|^2)^2\omega^2}\right)\omega-\frac{-4(\alpha_n+\eta_n|\bar{b}|^2)\omega|\psi_n||\bar{b}|}{\sqrt{\left(2\omega-\omega_n-\Psi_n|\bar{b}|^2\right)^2+4(\alpha_n+\eta_n|\bar{b}|^2)^2\omega^2}}\right)^2\right\}\times$$
$$\frac{|\bar{b}|}{|\psi_n|}\sqrt{\left(2\omega-\omega_n-\Psi_n|\bar{b}|^2\right)^2+4(\alpha_n+\eta_n|\bar{b}|^2)^2\omega^2}=\zeta^2 \tag{16}$$

After numerically solving Eq. (16) for $|\bar{b}|$, and using it in Eq. (12), we can calculate the amplitude of the quasi-uniform mode $|\bar{a}|$.

## III. EFFECTS OF THE DRIVE AMPLITUDE AND INTRINSIC NONLINEARITITES

To understand the impact of the intrinsic nonlinearity parameters ($\Psi_0$, $\Psi_n$, $\eta_0$, $\eta_n$) on the quasi-uniform spin wave mode resonance, we plot the numerical solution of Eq. (16) in Supplemental Figure 2. Each panel of this figure shows a reference lineshape of the resonance calculated with all intrinsic nonlinearity parameters set to zero (red curve) and a lineshape calculated with one of the intrinsic nonlinearity parameter different from zero (blue curve). This figure reveals that increasing $\eta_0$ decreases the mode amplitude and slightly increases the linewidth. Increasing $\eta_n$ decreases the degree of the double-peak lineshape splitting. Increasing $\Psi_n$ increases the lineshape asymmetry. Increasing $\Psi_0$ increases lineshape asymmetry and induces fold-over.

Supplemental Figure 3 shows the linewidth as a function of the drive amplitude for three scenarios, where the intrinsic nonlinearities $\Psi_0$, $\Psi_n$, $\eta_0$, $\eta_n$ are set to zero for simplicity. If the coupling parameter is zero, $\psi_n = 0$, the linewidth does not depend on the drive amplitude, as expected for a single-mode linear oscillator. The second case demonstrates that the linewidth remains constant when the product $\psi_n \cdot \zeta$ is constant. For a constant non-zero coupling parameter, the linewidth shows an increase with the drive amplitude. This observation allows us to employ a single fitting parameter ($\psi_n \cdot \zeta$) to fit the data in Fig. 1b. This conjecture can be confirmed analytically by introducing a normalized spin wave amplitude $\hat{a} = \psi_n \bar{a}$, which allows us to rewrite Eq. (16) omitting all intrinsic nonlinearities into the following form:

$$\omega\left[1+i\alpha_0+i\frac{4\alpha_n|\hat{a}|^2}{(2\omega-\omega_n)^2+4\alpha_n^2\omega^2}\right]\hat{a}-\omega_0\hat{a}-\frac{2(2\omega-\omega_n)}{(2\omega-\omega_n)^2+4\alpha_n^2\omega^2}|\hat{a}|^2\hat{a}=\psi_n\zeta \tag{17}$$

This equation describes an effective single-mode nonlinear oscillator with renormalized excitation amplitude $\psi_n\zeta$.

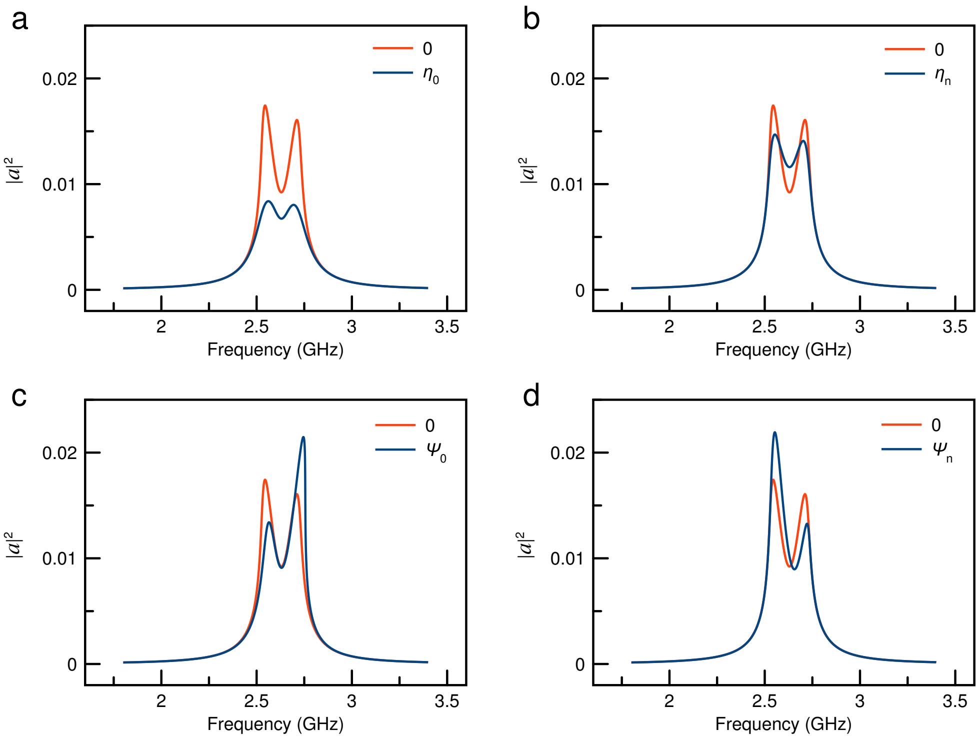


Supplemental Figure 2. Effect of intrinsic nonlinearities on the quasi-uniform spin wave resonance lineshape. Spectral lineshape of the quasi-uniform spin wave mode resonance $|\bar{a}|^2(\omega)$ at the three-magnon resonance condition $2\omega_0 = \omega_n$ calculated by numerically solving Eq. (16). The red curve is a reference lineshape calculated with all intrinsic nonlinearity parameters $(\eta_0, \eta_n, \Psi_0, \Psi_n)$ set to zero. The blue lineshape in each panel is calculated with one of the intrinsic nonlinearity parameters set to a non-zero value: (a) $\eta_0 = 1.325 \cdot 10^{-24}$ J, (b) $\eta_n = 3.313 \cdot 10^{-24}$ J, (c) $\Psi_0 = 1.325 \cdot 10^{-24}$ J, (d) $\Psi_n = 1.325 \cdot 10^{-23}$ J. Other parameters employed in the calculation are: $\omega_0 = 2\pi \cdot 2.63\,\text{GHz}$, $\omega_n = 2\pi \cdot 5.26\,\text{GHz}$; $\alpha_0 = 0.02662$, $\alpha_n = 0.03042$ at $I_{\text{dc}} = 0$; $\psi_n \cdot \zeta = h^2 \cdot 0.006\,\text{GHz}^2$, where $h$ is the Planck constant.

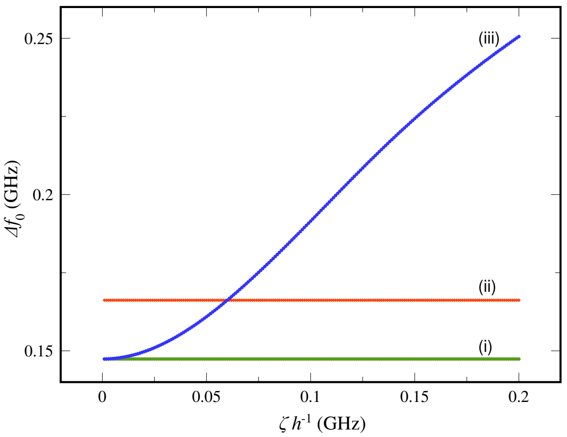


Supplemental Figure 3. Effect of the drive amplitude on linewidth in the resonant three-magnon regime. Calculated linewidth of the quasi-uniform spin wave mode as a function of the drive amplitude $\zeta$ for different values of the mode coupling parameter $\psi_n$. (i) Green: $\psi_n = 0$, (ii) red: variable $\psi_n$ with a constraint $\psi_n \cdot \zeta = h^2 \cdot 0.006\,\text{GHz}^2$, and (iii) blue: $\psi_n = h \cdot 0.1\,\text{GHz}$. All intrinsic nonlinearity parameters: $\Psi_0$, $\Psi_n$, $\eta_0$ and $\eta_n$ are set to zero. $h$ is the Planck constant. Other parameters employed in the calculation are: $\omega_0 = 2\pi \cdot 2.63\,\text{GHz}$, $\omega_n = 2\pi \cdot 5.26\,\text{GHz}$; $\alpha_0 = 0.02662$ and $\alpha_n = 0.03042$ at $I_{\text{dc}} = 0$.

## IV. EFFECTIVE SINGLE-MODE NONLINEAR OSCILLATOR APPROXIMATION

If we neglect intrinsic nonlinearities $\Psi_n$ and $\eta_n$ of the higher order spin wave mode, Eq. (16) can be reduced to a cubic equation for $\bar{a}$ and solved analytically. This approximation allows us to obtain several important qualitative insights into the properties of the resonant nonlinear damping of the quasi-uniform mode. By setting $\Psi_n = 0$ and $\eta_n = 0$ in Eq. (8), we obtain an exact solution for $\bar{b}$:

$$\bar{b} = \frac{\psi_n^* \bar{a}^2}{2\omega(1 + i\alpha_n) - \omega_n} \tag{18}$$

Using this result, we reduce Eq. (16) to a cubic algebraic equation for $\bar{a}$:

$$\omega \left[ 1 + i(\alpha_0 + \eta_0 |\bar{a}|^2) + i \frac{4|\psi_n|^2 \alpha_n |\bar{a}|^2}{(2\omega - \omega_n)^2 + 4\alpha_n^2 \omega^2} \right] \bar{a} - \omega_0 \bar{a} - \left[ \Psi_0 + \frac{2|\psi_n|^2 (2\omega - \omega_n)}{(2\omega - \omega_n)^2 + 4\alpha_n^2 \omega^2} \right] |\bar{a}|^2 \bar{a} = \zeta \tag{19}$$

This equation describes the amplitude $\bar{a}$ of an effective single-mode nonlinear oscillator.

It is evident from Eq. (19) that the frequency of the quasi-uniform mode experiences a nonlinear shift:

$$\omega_0^{\text{eff}} = \omega_0 + \left[ \Psi_0 + \frac{2|\psi_n|^2 (2\omega - \omega_n)}{(2\omega - \omega_n)^2 + 4\alpha_n^2 \omega^2} \right] |\bar{a}|^2 \tag{20}$$

The nonlinear frequency shift has a well-pronounced antisymmetric resonant character near the resonance frequency $\omega_n/2$, that arises from the resonant three-magnon scattering.

Further, it is clear from Eq. (19) that the effective damping of the quasi-uniform mode also acquires a term arising from the three-magnon interaction:

$$\alpha_0^{\text{eff}} = \alpha_0 + \left[ \eta_0 + \frac{4|\psi_n|^2 \alpha_n}{(2\omega - \omega_n)^2 + 4\alpha_n^2 \omega^2} \right] |\bar{a}|^2 \tag{21}$$

The last term describes a resonant enhancement of the nonlinear damping by three-magnon scattering near the resonance frequency $\omega_n/2$. Strikingly, the magnitude of the resonant damping enhancement at $\omega_n/2$ increases when the intrinsic damping of the higher order mode $\alpha_n$ decreases. In the limit $\alpha_n \to 0$, the effective damping becomes

$$\alpha_0^{\text{eff}} \to \alpha_0 + \left[ \eta_0 + \frac{2\pi |\psi_n|^2}{\omega} \delta(2\omega - \omega_n) \right] |\bar{a}|^2 \tag{22}$$

where $\delta$ is Dirac's delta function. Equation (21) suggests that the effective damping of the quasi-uniform mode $\alpha_0^{\text{eff}}$ can increase with increasing antidamping spin torque applied to the nanomagnet. Indeed, the antidamping spin torque tends to increase the amplitude [6] of the quasi-uniform mode $|\bar{a}|$ and decrease the intrinsic damping parameter of the higher order mode $\alpha_n \to \alpha_n(1 - I_{\text{dc}}/I_{\text{c}}^{|n\rangle})$, both enhancing the nonlinear damping term in Eq. (19). For a sufficiently large mode coupling parameter $\psi_n$, the enhancement of the nonlinear damping term by the antidamping spin torque can exceed the reduction of the linear damping parameter $\alpha_0 \to \alpha_0(1 - I_{\text{dc}}/I_{\text{c}}^{|0\rangle})$ by the torque, leading to an increase of $\alpha_0^{\text{eff}}$ by $I_{\text{dc}} > 0$ and broadening of the quasi-uniform mode resonance by the antidamping spin torque. This scenario is indeed realized in the MTJ devices studied here as demonstrated by the data and calculations in Fig. 3.

## V. MODE COUPLING PARAMETER

In this Supplementary Note, we discuss how the coupling parameter between the spin wave modes, $\psi_n$ in Eq. (3), can be calculated. We consider a very thin, magnetically soft ferromagnetic disk with elliptical cross section, that is magnetized in-plane. Within a classical micromagnetic model, we include Zeeman, dipolar and exchange terms in the free energy. An applied field $H$ along the $x$ direction (long axis of the ellipse) magnetizes the sample to a nearly uniform state. Through a classical Holstein-Primakoff transformation [7] we introduce variables $c(\vec{x}, t)$ and $c^*(\vec{x}, t)$ to describe the magnetization such that the magnetization magnitude is conserved:

$$m_x = 1 - cc^* \ \ , \ \ m_+ = c\sqrt{2 - cc^*} \ \ , \ \ m_- = c^* \sqrt{2 - cc^*} \ , \tag{23}$$

where $\vec{m} = \vec{M}/M_s$, and $m_\pm \equiv m_z \pm i m_y$. Approximating the exchange energy to the fourth order in $c$ and $c^*$, the normalized free energy of the disk, $U \equiv E/4\pi M_s^2$, is given by

$$U \simeq -h_x \int (1 - cc^*)\, \mathrm{d}V + (l_{ex})^2 \int \left[ \vec{\nabla} c \cdot \vec{\nabla} c^* + \frac{1}{4} c^2 (\vec{\nabla} c^*)^2 + \frac{1}{4} c^{*2} (\vec{\nabla} c)^2 \right] \mathrm{d}V - \frac{1}{2} \int \mathrm{d}V \vec{h}_D(\vec{m}) \cdot \vec{m} \ , \tag{24}$$

with $h_x \equiv H/4\pi M_s$, $l_{ex} \equiv \sqrt{A/2\pi M_s^2}$ is the exchange length, and $\vec{h}_D(\vec{m}) = \vec{H}_D(\vec{m})/4\pi M_s$ is the normalized demagnetizing field. The Landau-Lifshitz equations of motion in the new variables are: $i\dot{c} = \delta U/\delta c^*$, $i\dot{c^*} = -\delta U/\delta c$ with $t' = 4\pi M_s|\gamma|t$.

Assuming the normal modes involved in three magnon scattering dominate the magnetization dynamics, the free energy in Eq. (24) can be written in terms of amplitudes of these modes, by expressing $c$ in terms of $a$ and $b$:

$$c(\vec{x},t) \simeq a(t)f(\vec{x}) + a^*(t)g(\vec{x}) + b(t)p(\vec{x}) + b^*(t)q(\vec{x}) \tag{25}$$

The functions $f, g, p, q$ can be determined from calculating the linear modes of oscillation of the sample. The terms of the free energy proportional to $aab^*$ and $a^*a^*b$ describe the three-magnon process and the magnitude of these terms gives the coupling parameter $\psi_n$.

If the magnetization state is approximated as exactly uniform, the dipolar energy for a very thin film may be approximated as $U_D = m_z^2/2 = (c+c^*)^2(1-cc^*/2)$, and in this case all three-magnon terms are zero. However, when the effects due to the sample edges (such as spatial inhomogeneity of the demagnetization field and edge roughness) are taken into account, the equilibrium magnetization configuration is generally nonuniform. In this case, there are non-zero three-magnon terms in the free energy expression. An explicit calculation of the corresponding overlap integrals is necessary for a quantitative prediction of $\psi_n$. Refs. [8, 9] show such extensive calculations for circular disks and include explicit expressions for the exchange and dipolar energies.


[1] Michael Harder, Yongsheng Gui, and Can-Ming Hu, "Electrical detection of magnetization dynamics via spin rectification effects," Phys. Rep. **661**, 1–59 (2016).

[2] A. M. Gonçalves, I. Barsukov, Y.-J. Chen, L. Yang, J. A. Katine, and I. N. Krivorotov, "Spin torque ferromagnetic resonance with magnetic field modulation," Appl. Phys. Lett. **103**, 172406 (2013).

[3] M. J. Donahue and D. G. Porter, *OOMMF User's Guide* (National Institute of Standards and Technology, Gaithersburg, MD, 1999).

[4] Robert D. McMichael and Mark D. Stiles, "Magnetic normal modes of nanoelements," J. Appl. Phys. **97**, 10J901 (2005).

[5] P. S. Keatley, V. V. Kruglyak, A. Neudert, R. J. Hicken, V. D. Poimanov, J. R. Childress, and J. A. Katine, "Resonant enhancement of damping within the free layer of a microscale magnetic tunnel valve," J. Appl. Phys. **117**, 17B301 (2015).

[6] J. C. Sankey, P. M. Braganca, A. G. F. Garcia, I. N. Krivorotov, R. A. Buhrman, and D. C. Ralph, "Spin-transfer-driven ferromagnetic resonance of individual nanomagnets," Phys. Rev. Lett. **96**, 227601 (2006).

[7] T. Holstein and H. Primakoff, "Field dependence of the intrinsic domain magnetization of a ferromagnet," Phys. Rev. **58**, 1098–1113 (1940).

[8] D. Mancilla-Almonacid and R. E. Arias, "Instabilities of spin torque driven auto-oscillations of a ferromagnetic disk magnetized in plane," Phys. Rev. B **93**, 224416 (2016).

[9] D. Mancilla-Almonacid and R. E. Arias, "Spin-wave modes in ferromagnetic nanodisks, their excitation via alternating currents and fields, and auto-oscillations," Phys. Rev. B **95**, 214424 (2017).
